# Supplementary material for: A Framework for Generating Explanations from Temporal Personal Health Data
Source: arXiv:2003.09530 source file (2021-03-10)
Supplement: Supplementary file 2 [file response.tex]

% LaTeX rebuttal letter example. 
% 
% Copyright 2019 Friedemann Zenke, fzenke.net
%
% Based on examples by Dirk Eddelbuettel, Fran and others from 
% https://tex.stackexchange.com/questions/2317/latex-style-or-macro-for-detailed-response-to-referee-report
% 
% Licensed under cc by-sa 3.0 with attribution required.

\documentclass[11pt]{article}
\usepackage[utf8]{inputenc}
\usepackage{lipsum} % to generate some filler text
\usepackage{fullpage}

% import Eq and Section references from the main manuscript where needed
% \usepackage{xr}
% \externaldocument{manuscript}

% package needed for optional arguments
\usepackage{xifthen}
% define counters for reviewers and their points
\newcounter{reviewer}
\setcounter{reviewer}{0}
\newcounter{point}[reviewer]
\setcounter{point}{0}

% This refines the format of how the reviewer/point reference will appear.
\renewcommand{\thepoint}{P\,\thereviewer.\arabic{point}} 

% command declarations for reviewer points and our responses
\newcommand{\reviewersection}{\stepcounter{reviewer} \bigskip \hrule
                  \section*{Reviewer \thereviewer}}

\newenvironment{point}
   {\refstepcounter{point} \bigskip \noindent {\textbf{Reviewer~Point~\thepoint} } ---\ }
   {\par }

\newcommand{\shortpoint}[1]{\refstepcounter{point}  \bigskip \noindent 
	{\textbf{Reviewer~Point~\thepoint} } ---~#1\par }

\newenvironment{reply}
   {\medskip \noindent \begin{sf}\textbf{Reply}:\  }
   {\medskip \end{sf}}

\newcommand{\shortreply}[2][]{\medskip \noindent \begin{sf}\textbf{Reply}:\  #2
	\ifthenelse{\equal{#1}{}}{}{ \hfill \footnotesize (#1)}%
	\medskip \end{sf}}

\begin{document}

\section*{Response to the reviewers}
% General intro text goes here

We thank the reviewers for the valuable feedback and comments on
our manuscript. 
We have thoroughly revised our manuscript to address most of the
concerns that were raised. 
We have significantly expanded the manuscript so that the novelty and
significance of our work is more clear. 
Our work significantly expands the literature on linguistic summaries by
handling time-series data in a more comprehensive manner than existing
works.

Major new items in the revision include the generation of explanatory data provenance
charts that help support the natural language summaries.
Also new is a user study to
evaluate the effectiveness, usefulness and comprehensibility of our
generated summaries. All major new content is colored
in blue font so the reviewers can clearly discern our changes. 
We believe that the paper is much stronger as a result of the changes.
We detail our responses on specific points below.

% Let's start point-by-point with Reviewer 1
\reviewersection

% Point one description 
\begin{point}
	They describe the framework design as a contribution, and, at the same time, have a strong focus on the specifics of a certain application. Neither of these parts seems
properly evaluated. In case the framework is the contribution, I would like to see a deeper discussion of
design alternatives. If the application is in the focus, then there is a need to evaluate the outputs of the
system more thoroughly.
	\label{pt:hierarchy}
\end{point}

% Our reply:
\begin{reply}
Our protoform framework is a major
contribution of the work. Indeed, we explored several different ways to
characterize the protoforms, before eventually converging to the one in
Fig 2. For example, our first attempts focused on the pattern types such
as tendencies, observations, goal assessments and shape-based. Another
approach was based on the computational approach, such as ratio-based,
SAX-based, shape-based, sequence-based, etc. The hierarchy reported in
the paper was a result of careful crafting over a period of 1-2 years,
and incorporates the main ideas from the earlier attempts.

Besides the protoforms, our major focus in on understandability. For
this reason, we have enhanced our revision with summary provenance
charts that were in turn inspired by the user study to judge the
efficacy of our framework in terms of comprehensibility, usefulness and
data alignment.

We also show that the framework is generalizable, by including summaries
generated from Weather and Stock Market data.
\end{reply}

\begin{point}
	There must be at least
some initial form of a user-centric evaluation of the framework. I could imagine that at least some study
is done where, e.g., external evaluators assess in a systematic way to what extent the results produced
by the system are actually meaningful and correct and/or helpful for end users.
	\label{pt:eval}
\end{point}

\begin{reply}
    We thank the reviewer for this suggestion. As noted above, our
    revised manuscript now includes a user study comprising human
    evaluation of our summaries
    on meaningfulness, helpfulness, and correctness. 
    Details of the user study are in Sec 5.4.
In brief, the preliminary user study confirms that our approach is
indeed effective and useful. However, it also elucidated aspects that
need improvement.
\end{reply}


\begin{point}
	The various parameters of the framework in my view are in fact a challenging problem. No guidance is
given by the authors how to select them. Sometimes they refer to ``standard'' values, but it is not clear
where the standards come from and why these settings should be meaningful in general. Is there any
better way than trial-and-error to find parameters for a given application?
	\label{pt:parameters}
\end{point}

\begin{reply}
    We have now added more discussion on how to choose the different
    parameters in Section 5.2 in the revised manuscript. We discuss there the
    effect of the choices for the time window, alphabet size, and
    support and confidence thresholds, including how to choose them.
\end{reply}

\begin{point}
	Limitations of the work should be discussed as well. Some limitations are mentioned (e.g., that some
engineering effort is required), but I think there are more challenges,
e.g., regarding the tuning of the parameters or the fact that the system does not learn beyond what was hard-coded as rules.
	\label{pt:limitation}
\end{point}

\begin{reply}
	A  limitation of our approach is that it is
    confined to its rules, so we state this in the Conclusions and
    add to the discussion of limitations throughout the
    paper.   The discussion of parameters was added to Sec 5.2, as noted
    above.
\end{reply}

\begin{point}
    More evidence would be helpful that shows that the summary metrics are actually useful. The rationale
of these metrics could also be better explained in the text. Table 3 and other tables show some values
for the metrics, but no explanation is provided. Are these values good? What is the range of values?
\label{pt:metrics}
\end{point}

\begin{reply}
    We have clarified and added more details  on how the metrics are
    computed. The various minor changes are not highlighted in blue, but
    the text has been updated in section 4.2. 
    We have also added a length quality evaluation metric to evaluate
    the length of our summaries, we have stated the ranges for each metric and described the ideal value of those metrics. Finally, we added in more details regarding the usefulness of the metrics and what they mean for the summaries.
\end{reply}

\begin{point}
    I propose to discuss previous works first. It should also be explicitly mentioned early on
that the system is built on existing technical approaches. The discussion of related works seems a bit shallow, given also that many technical components of the
framework are based on existing works. I also recommend to clearly start with a statement that principles of the work of Zadeh were
adopted here.
\label{pt:relatedworks}
\end{point}

\begin{reply}
    We have restructured the paper by placing the Related Works section
    right after the Introduction in Sec 2. 
    We have also added more details of related works, and clearly
    mentioned the work we build upon, including Zadeh's seminal work.
\end{reply}

\begin{point}
    In Section 2, the authors state that they aim to generate a set of diverse explanations
(summarizations), but a motivation why diversity is important here, or how diversity is assessed is
missing.
\end{point}

\begin{reply}
    In terms of the importance of having diversity in our summaries, we
    explain in Section 3 about how each of the summary types provides a
    different way to look at the data for a user. Indeed, the addition
    of the summary provenance provides intuitive justification for the
    various types of protoforms we define. 
    We describe the summaries from the perspective
of a user who is exploring their data looking for summaries from the
simple to the more complex, which further
motivates the need for each summary type.
\end{reply}

\begin{point}
    I was wondering what happens in a practical application, when the system is not available to produce
a summarization with the given thresholds. What would that mean for the user ‐ would we show that no
trend was detected?
\end{point}

\begin{reply}
    While our framework provides the protoforms, different applications
    will require some parameter tuning to generate useful results. We
    have added such discussion in Sec 5.2 as noted above.
\end{reply}

\subsection*{Minor}

\begin{point}
    ``The user can use the following protoform with S''. Who is the ``user'' here? I don't think end users
would use protoforms.
\end{point}

\begin{reply}
    To address some confusion with the ``user'' of the protoforms, we took those phrases out since the target user (the non-expert looking at the data) does not interact with the protoforms; rather, they interact with the resulting summaries. If anything, a clinician or physician could hypothetically interact with the protoforms if they wish to find certain patterns in the data.
\end{reply}

\begin{point}
    Are there any insights from the literature what would be considered too
lengthy? Considering the example ``In week 11, your calorie intake was moderate, then very low, then
high, then very high, then low, then moderate. During'', I would already think this is too long.
\end{point}

\begin{reply}
    We have added in a length quality metric to address this issue and to evaluate our summaries accordingly.
\end{reply}

\begin{point}
    ``Example: In order to better to follow the 2000-calorie diet, you should decrease your calorie intake.'' This rule does not seem very meaningful.
\end{point}

\begin{reply}
    We agree with the reviewer and mention in the paper that the diet we have chosen shows more about the potential capabilities of goal assistance summaries with more complex diets.
\end{reply}

\begin{point}
    ``Some of the users in this study had a moderate calorie intake in the past full week.'' I wonder why
such an information should be interesting to a user.
\end{point}

\begin{reply}
    We agree and we believe that researchers and/or clinicians would be
    more interested in this kind of summary. We have added this explanation into the paper in Section 3.4.
\end{reply}

% Use the short-hand macros for one-liners.
\shortpoint{ The title/abstract of the paper suggest that this work is about explanations, but it is about text
summarization. }
\shortreply{ We have changed “explanations” to “summaries” for the most part since, although they do have the capability to explain, they are not used that way in this context.}

\shortpoint{ Some references seem incomplete. }
\shortreply{ We have looked through our references and updated any that seemed incomplete. }

\shortpoint{The quality of Figure 2 could be improved.}
\shortreply{We have improved the visuals of each (sub-)hierarchy.}

\shortpoint{Typo: ``dataset D. i The goal''}
\shortreply{Fixed.}
% Begin a new reviewer section
\reviewersection

\begin{point}
	Setting the values of the input parameters of the sequence mining and clustering algorithms could be challenging. This points requires further discussion and explanations.
\end{point}

\begin{reply}
	We address this point in response to \ref{pt:parameters}.
\end{reply}

\begin{point}
The sequence mining algorithm could extract sequences in which a time gap may occur between prefix and suffix. Have you enforced any constraint in SPADE on the gap duration, number of occurring items per time span, and occurrence of other items in-between? Why not using the simpler association rule mining framework to address the same problem while dealing with consecutive time windows?
\end{point}

\begin{reply}
For if-then patterns, we do not explicitly use time gaps, although, our
data can have ``natural'' gaps, i.e., since the measurements are not
always on all consecutive days, and there can be missing days in the
data. These are manifested in the day-based patterns. In the future, we
plan to handle these natural gaps via appropriate settings within SPADE.
For consecutive pattern mining we can certainly use other methods;
ultimately, our focus is more on the interesting and useful summary
types, and we will use the best methods for the task. Finally, note that
we are using sequential association rules as described in Sec 4.1 (we do
need order information, so we cannot a pure item-set based approach in
regular association rules).
\end{reply}

\begin{point}
Qualitative feedback from real users (collected through a survey) would be more effective in evaluating the actual usability and effectiveness of the system.
\end{point}

\begin{reply}
We have addressed this point in response to \ref{pt:eval}.
\end{reply}

\begin{point}
What is the relationship between the degree of appropriateness and support/confidence of a if-then pattern? Since they seem to be correlated with each other, the use of that particular quality metrics appeared to be inappropriate.
\end{point}

\begin{reply}
    Degree of appropriateness is a different (fuzzy) metric for
    measuring the significance of a summary based on sub-summaries. It
    is different from confidence and support in that respect. 
\end{reply}

\begin{point}
The average membership function is user-provided. Could it be inferred automatically from past user experience data?
\end{point}

\begin{reply}
In principles this is possible, if different user can provide feedback
in the form of the quantifier labels, e.g., when would they consider
something to be ``most of the''. If we had these values for different
users, we could infer the membership function. However, as defined, the
fuzzy membership functions are already designed to capture the inherent
vagueness in those labels, as can be seen in the new Fig.~20.
\end{reply}

\begin{point}
The portability of the systems towards multilingual context should be discussed as well.
\end{point}

\begin{reply}
We believe that this is an interesting direction, but quite beyond the
scope of our current work.
\end{reply}
\end{document}
